# Supplementary material for: AutoMLP: Automated MLP for Sequential Recommendations
Source: arXiv:2303.06337 source file (2023-03-11)
Supplement: Supplementary file 1 [file 7_Appendix.tex]

\begin{table}
    % \centering
 \caption{Best hyper-parameter results}
 \label{table:statistics}
 \begin{tabular}{@{}|c|c|c|c|c|}
  \hline
  Model & Dataset & embedding size & hidden size & layers \\ \hline
  \ \multirow{2}{*}{FPMC} & MoiveLens & 128 & - & - \\
  \ & Beauty & 128 & - & - \\
  \ \multirow{2}{*}{GRU4Rec} & MoiveLens & 128 & 256 & 1 \\
  \ & Beauty & 128 & 256 & 1 \\
  \ \multirow{2}{*}{BERT4Rec} & MoiveLens & 128 & 512 & 2 \\
        \ & Beauty & 64 & 128 & 2 \\
  \ \multirow{2}{*}{NextItNet} & MoiveLens & 64 & - & -  \\
  \ & Beauty & 64 & - & - \\
  \ \multirow{2}{*}{GUR4Rec$^+$} & MoiveLens & 128 & 256 & 1 \\
  \ & Beauty & 128 & 256 & 1 \\
  \ \multirow{2}{*}{FDSA} & MoiveLens & 128 & 512 & 2 \\
  \ & Beauty & 128 & 512 & 2 \\
%   \ \multirow{2}{*}{MLP-Mixer} & MoiveLens & 128 & 512 & 4 \\
%   \ & Beauty & 128 & 512 & 4 \\
  \ \multirow{2}{*}{AutoMLP} & MoiveLens & 128 & 512 & 4 \\
  \ & Beauty & 128 & 512 & 10 \\ \hline
 \end{tabular}
 \vspace{-2.1mm}
\end{table}

\section{Reproduction Guidelines}
\label{sec:guide}

In this section we will mainly introduce how to reproduce our experimental results from RecBole~\cite{zhao2021recbole} - a comprehensive recommender system library based on Pytorch, enabling fast and easy reproduction in a fair environment. Before downloading and decompressing our code, please first make sure that you have followed the install guidelines of RecBole.
% \footnote{https://github.com/RUCAIBox/RecBole}. 
Note that to prevent unexpected errors, you should download the latest version, \ie 1.0.0 up till now. For the same reason, please make sure that you have the Pyotrch in version 1.9.0
% \footnote{https://pytorch.org/get-started/previous-versions/}
, and to enable GPU acceleration, you should have a cuda-capable system with cuda version 11.5.

Once RecBole is installed, find our submitted code in Dropbox, and replace your installed RecBole with our code. 

Please note that our experiments are conducted on NVIDIA Tesla V100S, for full reproduction we recommend you to use the same device, otherwise due to the accumulations of different float operations, we cannot make the guarantee for reproducing same results.
% \footnote{https://discuss.pytorch.org/t/different-machines-different-results/100126}.

To run experiments, please refer to RecBole's manual for quick start,
% \footnote{https://recbole.io/docs/get$\_$started/quick$\_$start.html}
procedures for running our code are similar. Please note that if you wish to reproduce AutoMLP's results, use model named "MLP", you can find the detailed code implementation under the  "RecBole/recbole/model/sequential$_$recommender/mlp.py". If you wish to reproduce the short-term interest length search, run model named "AutoMLP", once weights are converged, use searched result for "MLP".

Due to file size limits, we did not include any data we used in experiments. If you wish to reproduce any experiments, please refer to RecBole dataset site~\cite{zhao2021recbole}
% \footnote{https://recbole.io/dataset$\_$list.html} 
for usage guidelines. 

%remove_private_20220607
% Notably, the NetEase Game dataset is private data. Due to company policies, it is strictly limited for internal utilization. However relevant evidence such as snapshot or original log of experiment results could be provided if required. 

\section{Hyper-parameter Tuning}
\label{sec:hyper}
In this section we give the search space of hyper-parameters of our baseline models. We apply common techniques to prevent over-fitting such as weight decay and dropout, for generality, the dropout is set to be 0.5 for all baselines. We search weight decay for all methods in \{0,1e-2,1e-3\}, embedding size in \{32,64,128,256\}, hidden unit size in \{128,256,512\}, and number of layers in \{1,2,4,6,8,10,12\}. Specifically, we set the number of self-attention heads in BERT4Rec and FDSA according to the recommendation of original paper \cite{sun2019bert4rec}. The kernel size of NextItNet is set as 3. The fine-tuned hyper-parameters results are shown in Table \ref{table:statistics}.
